# Supplementary material for: When to Assist and What to Suggest: Joint Gating and Memory-Grounded Hint Generation in One Compact Decoder
Source: arXiv:2610.40611 source file (2026-10-29)
Supplement: Supplementary file 1 [file inline.tex]

\makeatletter
\NewDocumentCommand\suppinline{m}{%
  \par\addvspace{\intextsep}\noindent
  \begin{minipage}{\linewidth}\centering\def\@captype{#1}}
\NewDocumentCommand\suppinlineend{}{\end{minipage}\par\addvspace{\intextsep}}
\NewDocumentCommand\suppinlinefloats{}{%
  \RenewDocumentEnvironment{table}{o}{\suppinline{table}}{\suppinlineend}%
  \RenewDocumentEnvironment{table*}{o}{\suppinline{table}}{\suppinlineend}%
  \RenewDocumentEnvironment{figure}{o}{\suppinline{figure}}{\suppinlineend}%
  \RenewDocumentEnvironment{figure*}{o}{\suppinline{figure}}{\suppinlineend}}
\makeatother
\newcommand{\suppfigwidth}{0.42\textwidth}
